# Supplementary material for: Swimmer suspensions on substrates: anomalous stability and long-range order
Source: arXiv:1901.01069 ancillary file (2019-01-04)
Supplement: Supplementary file 1 [file SuperStablePolarSI.pdf]

# Swimmer suspensions on substrates: anomalous stability and long-range order: Supplementary information

Ananyo Maitra,[1, *] Pragya Srivastava,[2] M. Cristina Marchetti,[3] Sriram Ramaswamy,[4] and Martin Lenz[1, †]

[1] *LPTMS, CNRS, Univ. Paris-Sud, Université Paris-Saclay, 91405 Orsay, France*
[2] *The Francis Crick Institute, Lincoln's Inn Fields Laboratory, 44 Lincoln's Inn Fields, London WC2A 3LY*
[3] *Physics Department and Syracuse Soft Matter Program, Syracuse University, Syracuse, NY 13244, USA*
[4] *Indian Institute of Science, Bangalore 560012, India*

In this supplement we present the detailed calculations leading to the results of the main paper. Section I presents the calculation for the limit of stability of the disordered phase. Section II presents the dynamical equations for the polarisation field including the effects of anisotropic mobility and an anisotropic coupling between the polarisation and the velocity fields. Section III presents the dynamical matrix used to calculate $\kappa_\pm$ and $\kappa_c$ in the main paper. Section IV presents the detailed calculation of the static structure factor of concentration fluctuations deep in the ordered phase. We present the mapping of the Malthusian version of our model to equilibrium smectics in the section V. A standard mapping of this to the KPZ equation then yields the equal-time exponents of this model. Section VI demonstrates that an apolar model with the constraint $\nabla\nabla : \mathbf{Q} = 0$ is not equivalent to a nematic in an incompressible fluid. Section VII explicitly displays the thickness averaging of a polar active fluid confined in a channel. Finally, in section VIII we show that our calculations are relevant for even compressible systems provided they are dense enough.

## I. INSTABILITY OF THE DISORDERED PHASE

In this section we calculate the limit of stability of the disordered state. The dynamical equations of motion for polarisation and velocity are

$$\partial_t \mathbf{p} = \Lambda \mathbf{u} - \frac{\delta \mathcal{H}}{\delta \mathbf{p}} \tag{1}$$

and

$$\Gamma \mathbf{u} = \upsilon \mathbf{p} - \nabla \Pi - \Lambda \frac{\delta \mathcal{H}}{\delta \mathbf{p}}. \tag{2}$$

Using $\mathcal{H}$ from the main text and expanding about a state with $\mathbf{p} = \mathbf{u} = 0$, we have

$$\partial_t \delta \mathbf{p} = \Lambda \delta \mathbf{u} - \alpha \delta \mathbf{p} \tag{3}$$

$$\Gamma \delta \mathbf{u} = (\upsilon - \Lambda \alpha)\, \delta \mathbf{p} - \nabla \Pi \tag{4}$$

This implies

$$\partial_t \begin{pmatrix} p_x \\ p_y \end{pmatrix} = \begin{pmatrix} -\alpha + \frac{\Lambda}{\Gamma}(\upsilon - \Lambda\alpha)\frac{q_y^2}{q^2} & -\frac{\Lambda}{\Gamma}(\upsilon - \Lambda\alpha)\frac{q_x q_y}{q^2} \\ -\frac{\Lambda}{\Gamma}(\upsilon - \Lambda\alpha)\frac{q_x q_y}{q^2} & -\alpha + \frac{\Lambda}{\Gamma}(\upsilon - \Lambda\alpha)\frac{q_x^2}{q^2} \end{pmatrix} \begin{pmatrix} p_x \\ p_y \end{pmatrix} \tag{5}$$

which has the eigenvalues $-\alpha$ and

$$-\left[\alpha - \frac{\Lambda}{\Gamma}(\upsilon - \Lambda\alpha)\right] = -\left[\alpha\left(1 + \frac{\Lambda^2}{\Gamma}\right) - \frac{\Lambda\upsilon}{\Gamma}\right] \tag{6}$$

The disordered phase is destabilised when either of these eigenvalues are positive. For $\Lambda\upsilon > 0$, this happens when

$$\tilde{\alpha} = \alpha - w = \alpha - \left(1 + \frac{\Lambda^2}{\Gamma}\right)^{-1} \frac{\Lambda\upsilon}{\Gamma} = 0 \tag{7}$$

as pointed out in the main text.

## II. GENERAL DYNAMICAL EQUATIONS TO ORDER $\mathbf{q}^0$

In this section we look at generalisations of the equations of motion eq. (1) and eq (2) of the main paper. For simplicity, we will not consider the dynamics of concentration field here. In general, both $\Gamma$, and $\Lambda$ in eq (1) and (2) can be $2 \times 2$ matrices. In a phase ordered along $\hat{x}$, the matrices must be constructed from the identity tensor $\mathsf{I}$ and $\hat{x}\hat{x} - (1/2)\mathsf{I}$.

The general equations of motion are

$$\partial_t \mathbf{p} = \mathbf{\Lambda} \cdot \mathbf{u} - \frac{\delta \mathcal{H}}{\delta \mathbf{p}} \tag{8}$$

$$\mathbf{u} = \mathsf{M} \cdot \left[\upsilon \mathbf{p} - \nabla \Pi - \mathbf{\Lambda} \cdot \frac{\delta \mathcal{H}}{\delta \mathbf{p}}\right] \tag{9}$$

where the mobility tensor $\mathsf{M}$ is the inverse of the friction tensor $\mathbf{\Gamma}$: $\mathsf{M}^{-1} = \mathbf{\Gamma}$. The diagonal tensors are defined as

$$\mathsf{M} = \begin{pmatrix} m_1 & 0 \\ 0 & m_2 \end{pmatrix} \tag{10}$$

$$\mathbf{\Lambda} = \begin{pmatrix} \Lambda_1 & 0 \\ 0 & \Lambda_2 \end{pmatrix} \tag{11}$$

Considering an ordered state $\mathbf{p} = p_0\hat{x}$ and using the same free-energy as in the main text, we see that $p_0$ is given by the condition

$$\Lambda_1 \upsilon m_1 - \left(1 + m_1\Lambda_1^2\right)(\alpha + \beta p_0^2) = 0 \tag{12}$$

Writing

$$\mathbf{p} = p_0 \begin{pmatrix} 1 \\ 0 \end{pmatrix} + \begin{pmatrix} \delta p \\ p_0\theta \end{pmatrix} = p_0\hat{x} + \delta\mathbf{p}, \tag{13}$$

we can write the equations of motion for $\delta p$ and $\theta$:

$$\partial_t \delta p = \Lambda_1 \delta u_x - w\delta p - 2|\tilde{\alpha}|\delta p + K_p \nabla^2 \delta p, \tag{14}$$

where $w = \left(1 + m_1\Lambda_1^2\right)^{-1} \Lambda_1 \upsilon m_1$ and $\tilde{\alpha} = \alpha - w$ as in the main text, and

$$\partial_t \theta = \frac{\Lambda_2}{p_0}\delta u_y - w\theta + K_p\nabla^2\theta \tag{15}$$

Defining

$$\mathsf{S} = \begin{pmatrix} \upsilon - \Lambda_1 w - \Lambda_1 2|\tilde{\alpha}| & 0 \\ 0 & \upsilon - \Lambda_2 w \end{pmatrix} \tag{16}$$

the incompressibility constraint becomes

$$iq_i\delta u_i = 0 = iq_i M_{ij} S_{jk}\delta p_k + q_i M_{ij} q_j \Pi. \tag{17}$$

This implies that the pressure is

$$\Pi = \frac{-iq_i M_{ij} S_{jk} \delta p_k}{q_m M_{mn} q_n} \tag{18}$$

and

$$\delta u_i = M_{ij}\left[S_{jk}\delta p_k - \frac{q_j q_m M_{mn} S_{nr}\delta p_r}{q_s M_{st} q_t}\right]. \tag{19}$$

Writing $\mathbf{q} = q(\cos\phi\hat{x} + \sin\phi\hat{y})$, and inserting this into (14) and (15), we get, to zeroth order in gradients,

$$\partial_t \delta p = \left[\frac{\Lambda_1 m_1 m_2\{\upsilon - \Lambda_1(w + 2|\tilde{\alpha}|)\}}{m_1\cos^2\phi + m_2\sin^2\phi}\sin^2\phi\right]\delta p - \left[\frac{\Lambda_1 m_1 m_2 p_0(\upsilon - \Lambda_2 w)}{2(m_1\cos^2\phi + m_2\sin^2\phi)}\sin 2\phi\right]\theta - (w + 2|\tilde{\alpha}|)\delta p \tag{20a}$$

$$\partial_t\theta = \left[-w + \frac{\Lambda_2 m_1 m_2(\upsilon - \Lambda_2/w)}{m_1\cos^2\phi + m_2\sin^2\phi}\cos^2\phi\right]\theta - \left[\frac{\Lambda_2 m_1 m_2\{\upsilon - \Lambda_1(w + 2|\tilde{\alpha}|)\}}{2p_0(m_1\cos^2\phi + m_2\sin^2\phi)}\sin 2\phi\right]\delta p \tag{20b}$$

These equations reduce to eq. (4) of the main text (upon ignoring the concentration dynamics), when $\Lambda_1 = \Lambda_2 = \Lambda$, and $m_1 = m_2 = 1/\Gamma$. The detailed conditions for this to have two negative eigenvalues are rather complicated but both are certainly negative when $\Lambda_1$ and $\Lambda_2$ have the same sign as $\upsilon$ and $\Lambda_1 m_1 \geq \Lambda_2 m_2$.

## III. DYNAMICAL MATRIX FOR CALCULATION OF FLUCTUATIONS ABOUT AN ORDERED PHASE

The dynamical matrix for polarisation fluctuations $\delta\mathbf{p} = (p_0 + \delta p)(\cos\theta\hat{x} + \sin\theta\hat{y}) - p_0\hat{x}$ and concentration fluctuations $\delta c$, resulting from equations (1), (2) and (3) of the main text is

$$\partial_t \begin{pmatrix} \delta c \\ \delta p \\ \theta \end{pmatrix} = \begin{pmatrix} -D_c q^2 - i[\upsilon_p + w/\Lambda]p_0 q\cos\phi & -i\upsilon_p c_0 q\cos\phi & -i\upsilon_p c_0 p_0 q\sin\phi \\ \alpha_0' p_0 - i\gamma q\cos\phi & -2|\tilde{\alpha}|\{1 + \sin^2\phi\Lambda^2/\Gamma\} - w\cos^2\phi & -(wp_0/2)\sin(2\phi) \\ -i(\gamma/p_0)q\sin\phi & -\sin(2\phi)/(2p_0)\{w - 2|\tilde{\alpha}|\Lambda^2/\Gamma\} & -w\sin^2\phi - K_p(\phi)q^2 \end{pmatrix} \begin{pmatrix} \delta c \\ \delta p \\ \theta \end{pmatrix} \tag{21}$$

where $\alpha_0' = \partial_c\alpha|_{c=c_0} > 0$, $\phi$ is the angle between $\mathbf{q}$ and $\hat{x}$, and $K_p(\phi)$ is the effective Frank elastic coefficient whose explicit form is displayed in the next section. The eigenvalues of this matrix directly lead to the equations (6) and (7) of the main text. Advective and self-advective terms in the polarisation dynamics are not displayed here for clarity as they do not affect Eq. (6) and (7) of the main text. See the next section for the form of such terms.

## IV. CALCULATION OF THE STATIC STRUCTURE FACTOR OF CONCENTRATION FLUCTUATIONS

In this section, we present a detailed calculation of the static structure factor of concentration fluctuations deep in the ordered phase. To order to retain the correct angular dependence of the static structure factor, we first obtain the most general coupled equations for the concentration and angular fluctuations correct to $\mathcal{O}(q^2)$ deep in the ordered phase, after explicitly eliminating the velocity and the polarisation magnitude. For this, we extend the polarisation and the velocity equations, (1) and (2) of the main text, to include terms that affect the angular dynamics at $\mathcal{O}(q^2)$. The general equation for the polarisation field is [1]

$$\partial_t \mathbf{p} + \mathbf{u}\cdot\nabla\mathbf{p} + \lambda_a \mathbf{p}\cdot\nabla\mathbf{p} - \boldsymbol{\omega}\times\mathbf{p} = \Lambda\mathbf{v} - \lambda\mathbf{p}\cdot\mathbf{U} - \lambda_1\nabla^2\mathbf{v} - \frac{\delta\mathcal{H}}{\delta\mathbf{p}}, \tag{22}$$

where $\mathbf{U}$ is the symmetric part of $\nabla\mathbf{u}$, $\boldsymbol{\omega} = (1/2)\nabla\times\mathbf{u}$, $\lambda_a$ denotes the strength of active self-advection, $\lambda$ is flow-alignment parameter and $\lambda_1$ describes a higher-order flow-alignment term. The Stokes equation reads

$$\Gamma\mathbf{u} = \upsilon\mathbf{p} - \nabla\Pi + \zeta_p\nabla^2\mathbf{p} + \zeta_1\mathbf{p}\cdot\nabla\mathbf{p} + \zeta_2\mathbf{p}\nabla\cdot\mathbf{p} - \Lambda\frac{\delta\mathcal{H}}{\delta\mathbf{p}} - 2\lambda\nabla\cdot\left[\mathbf{p}\frac{\delta\mathcal{H}}{\delta\mathbf{p}}\right]^S - 2\nabla\cdot\left[\mathbf{p}\frac{\delta\mathcal{H}}{\delta\mathbf{p}}\right]^A + \lambda_1\nabla^2\frac{\delta\mathcal{H}}{\delta\mathbf{p}}, \tag{23}$$

where, as before, $\Pi$ enforces the incompressibility condition $\nabla\cdot\mathbf{u} = 0$ and superscripts $S$ and $A$ denote symmetric and antisymmetric parts of a tensor. $\zeta_1$ and $\zeta_2$ are independent since the dynamics does not conserve angular momentum due to the frictional couplng to the substrate [2]. $\zeta_p$ is another active term at second order in gradients. The equation for concentration is

$$\partial_t c + \mathbf{u}\cdot\nabla c = -\nabla\cdot(v_p c\mathbf{p} - D_c\nabla c). \tag{24}$$

where $D_c$ is the isotropic diffusivity.

We now eliminate the velocity field and the fluctuations of the polarisation magnitude to obtain the equation for angular fluctuations deep in the ordered phase $\mathbf{p} = p_0\hat{x}$:

$$\partial_t\theta = -i\frac{\gamma}{p_0}q_y\delta c - i\Lambda_a q_x\theta - K_p q^2\theta - w(\sin^2\phi)\theta \tag{25}$$

where

$$\Lambda_a = \left(\lambda_a + \frac{w}{\Lambda}\right)p_0 - \frac{wp_0}{2\Lambda}(1-\lambda\cos 2\phi) - \frac{\Lambda}{\Gamma}\left[\left(\zeta_1 + w\frac{1-\lambda}{2}\right)\cos^2\phi - \left(\zeta_2 - w\frac{1+\lambda}{2}\right)\sin^2\phi\right] \tag{26}$$

$$K_p = K + \frac{p_0}{2\Gamma}(1-\lambda\cos 2\phi)\left[\left(\zeta_1 + w\frac{1-\lambda}{2}\right)\cos^2\phi - \left(\zeta_2 - w\frac{1+\lambda}{2}\right)\sin^2\phi\right] + \left[\frac{1}{\Gamma}\left\{\Lambda\left(\zeta_p + \lambda_1 w + \Lambda K\right)\right\} - \lambda_1\frac{w}{\Lambda}\right]\cos^2\phi \tag{27}$$

and the one for concentration fluctuations is

$$\partial_t\delta c = -D_c q^2\delta c - iv_p c_0 p_0 q\sin\phi\theta - iv_p p_0 q\cos\phi\delta c - i\frac{w}{\Lambda}p_0 q\cos\phi\delta c \tag{28}$$

The mode-structure implied by (25) and (28) is

$$\omega_1 = -iw\sin^2\phi + \Lambda_a(\phi)\cos\phi q - i\left(K_p(\phi) - \frac{\gamma v_p c_0}{w}\right)q^2 \tag{29}$$

$$\omega_2 = \left(v_p + \frac{w}{\Lambda}\right)p_0\cos\phi q - i\left(D_c + \frac{\gamma v_p c_0}{w}\right)q^2 \tag{30}$$

To calculate the density correlator we introduce a nonconserving, Gaussian, zero-mean noise $\xi$ in (25), with the correlator

$$\langle\xi(\mathbf{q},\omega)\xi(\mathbf{q}',\omega')\rangle = B(2\pi)^3\delta^2(\mathbf{q}+\mathbf{q}')\delta(\omega+\omega'). \tag{31}$$

and a conserving, Gaussian, zero-mean noise $\xi_c$ to (28) with

$$\langle\xi_c(\mathbf{q},\omega)\xi_c(\mathbf{q}',\omega')\rangle = B_c(2\pi)^3 q^2\delta^2(\mathbf{q}+\mathbf{q}')\delta(\omega+\omega') \tag{32}$$

Defining

$$\begin{aligned} c_1(\phi) =&\Lambda_a(\phi)\cos\phi && (33a)\\ c_2(\phi) =&\left(v_p + \frac{w}{\Lambda}\right) p_0 \cos\phi && (33b)\\ D_1(\phi) =&w\sin^2\phi + \left(K_p(\phi) - \frac{\gamma v_p c_0}{w}\right) q^2 && (33c)\\ D_2(\phi) =&\left(D_c + \frac{\gamma v_p c_0}{w}\right) q^2 && (33d)\end{aligned}$$

the density correlator reads

$$\langle \delta c(\mathbf{q},\omega)\delta c(-\mathbf{q},-\omega)\rangle = \frac{v_p^2 c_0^2 p_0^2 q^2 B_\theta \sin^2\phi + [(\omega - c_1 q)^2 + (w\sin^2\phi + K_p q^2)^2] q^2 B_c}{[(\omega - c_1 q)^2 + D_1^2][(\omega - c_2 q)^2 + D_2^2]}, \tag{34}$$

which we integrate over $\omega$ to obtain the static-structure factor for small $q$:

$$S(\mathbf{q}) = \langle |\delta c(\mathbf{q},t)|^2\rangle = \int_\infty^\infty \frac{d\omega}{2\pi}\langle \delta c(\mathbf{q},\omega)\delta c(-\mathbf{q},-\omega)\rangle = \begin{cases} \dfrac{B_c w^2 \sin^4\phi + B v_p^2 c_0^2 p_0^2 \sin^2\phi}{\left(D_c + \frac{\gamma v_p c_0}{w}\right) w^2 \sin^2\phi}, & \text{for } \phi \neq 0\\ \dfrac{B_c}{D_c}, & \text{for } \phi = 0\end{cases} \tag{35}$$

Thus, $S(\mathbf{q}) \propto q^0$ for all wavevector directions. For $\phi \neq 0$, this is a direct consequence of superstability as discussed in the main text. The static structure factor in (35) does not diverge for $\mathbf{q} \to 0$ and the mean-squared number fluctuations, $\langle \delta N\rangle^2 = S(\mathbf{q} \to 0)\langle N\rangle$, scales as $\langle N\rangle$ just as in equilibrium systems.

## V. MAPPING TO AN EQUILIBRIUM SMECTIC

We now show that the mapping established by [9] between a polar fluid on a substrate with the constrain $\nabla\cdot\mathbf{p} = 0$ and a smectic is also obtained in our system, where $\mathbf{p}$ is not explicitly constrained but the velocity field $\mathbf{u}$ is incompressible, *i.e.*, $\nabla\cdot\mathbf{u} = 0$, in the simple case of a locally-fixed-concentration (Malthusian) flock [12]. Deep in the ordered phase, the $\delta p$ fluctuations relax much faster than the $\theta$ fluctuations and we only need to consider the dynamical equation for $\theta$. To find the nonlinearities that are relevant at large scales we first look at the linearised angular fluctuations in more detail. The linear equation for $\theta$ is

$$\partial_t\theta = -(w\sin^2\phi)\theta - K_p(\phi)q^2\theta + \xi, \tag{36}$$

where $\xi(\mathbf{r},t)$ is a zero-mean Gaussian white noise with $\langle \xi(\mathbf{r},t)\xi(\mathbf{r}',t')\rangle = 2B\delta(\mathbf{r}-\mathbf{r}')\delta(t-t')$, where $B$ is the strength of the noise. From this, we can calculate the equal-time correlator of the angular fluctuations:

$$\langle |\theta(\mathbf{q},t)|^2\rangle = \frac{Bq^2}{wq_y^2 + K_p(\phi)q^4} \tag{37}$$

where $K_p(\phi)$ is a renormalised Frank diffusivity (27). Even in the case where $K_p(\phi) > 0$ for all $\phi$, the angular fluctuations are highly anisotropic in the $\mathbf{q} \to 0$ limit: while they diverge as $1/q^2$ for $q_y \lesssim q_x^2$, they scale as $q^2/q_y^2 \ll 1/q^2$ for $q_y \gg q_x^2$. This implies that the fluctuations are most dominant in the vicinity of $\phi = 0$ and $\phi = \pi$, scaling as $1/q^2$. In this limit we can replace $K_p(\phi)$ by $K_p(0) = K_p$. To find the nonlinearities that can modify the linear scaling of angular fluctuations we use standard renormalisation group arguments and calculate which of them grow at large distances and long times if we rescale space, time and angle fields while keeping $w$, $B$, and $K_p$ constant. Rescaling $x \to bx$, $y \to b^\mu y$, $t \to b^z t$ and $\theta \to b^\chi\theta$, we find that the linear "anisotropy exponent" $\mu$, the linear "dynamical exponent" $z$ and the linear "roughness exponent" $\chi$ have to be 2, 2 and $-1/2$ respectively (see Ref. [9] for details).

We now project (22) transverse to itself to obtain the equation for $\theta$:

$$\partial_t\theta = \frac{\lambda_a}{p_0}(\sin\theta[\mathbf{p}\cdot\nabla\mathbf{p}]_x - \cos\theta[\mathbf{p}\cdot\nabla\mathbf{p}]_y) + \frac{1}{p_0}(\sin\theta[\mathbf{u}\nabla\mathbf{p}]_x - \cos\theta[\mathbf{u}\nabla\mathbf{p}]_y) - \frac{\Lambda}{p_0}(\sin\theta u_x - \cos\theta u_y) + \frac{1}{p_0}\left[\sin\theta\frac{\delta F}{\delta\mathbf{p}}_x - cos\theta\frac{\delta F}{\delta\mathbf{p}}_y\right], \tag{38}$$

where $[\mathbf{u}\nabla\mathbf{p}]$ contain all terms in (22) with one velocity, one polarisation and a gradient. The nonlinearities in Eq. (38) appear from two sources: 1 – velocity couplings of the form $[\mathbf{u}\nabla\mathbf{p}]$ and the self-advective term $\mathbf{p}\cdot\nabla\mathbf{p}$, the most

relevant of which scales as $q_y(\theta^2)_q$ in the regime $q_y \sim q_x^2$, where $(\theta^2)_q$ denotes the Fourier component of $\theta^2$ with the wavevector $q$, and 2 – Terms appearing due to the presence of the $\Lambda\mathbf{u}$ coupling which leads to nonlinearities of the form $(\theta^2)_q$ and $(\theta^3)_q$. Using the linear exponents, we see that all $(\theta^2)_q$ and $(\theta^3)_q$ nonlinearities grow under rescaling, and are thus relevant, while all nonlinearities at $\mathcal{O}(q)$ or higher are irrelevant. Retaining all relevant nonlinearities, the equation for angular fluctuations in Fourier space is thus

$$\partial_t\theta = w\sum_{k,m}\left[\frac{q_y}{q_x}\left(-\frac{q_y}{q_x}\theta_q + \frac{\theta_k\theta_{q-k}}{2}\right) - \theta_{q-k}\left(-\frac{k_x}{k_y}\theta_k + \frac{\theta_{k-m}\theta_m}{2}\right)\right] - K_p q_x^2\theta_q + \xi_q \tag{39}$$

By defining $\theta = \partial_x h$, this equation transforms into a standard equilibrium stochastic dynamics governed by a free-energy

$$F = (1/2)\int d^2\mathbf{r}[w(\partial_y h - (\partial_x h)^2/2)^2 + K_p(\partial_x^2 h)^2]. \tag{40}$$

This is the standard free-energy of a two-dimensional smectic. Following [9], we find the exact exponents $\chi = -1/2$ and $\mu = 3/2$ through a further mapping to the KPZ equation explained in detail there. The negativity of $\chi$ implies that the angular fluctuations decay exponentially fast with distance, implying that the ordered phase remains long-ranged even taking into account the effect of nonlinearities. Further, the fact that $\chi$ remains unchanged from its value in the linearised theory, even after taking into consideration the effects of nonlinearities, demonstrates that our conclusion regarding super-stability remains unmodified.

The equivalence we establish between Malthusian polar systems in an incompressible fluid and the model of Ref. [9] is extremely delicate. Malthusian *apolar* systems in an incompressible fluid are not equivalent to an apolar extension of Ref. [9], in which concentration fluctuations away from a spatiotemporally uniform state are severely penalised by a stiff potential, even at the linear level, as we show next. In addition, in a polar system with non-constant, yet conserved concentration, the concentration fluctuations are as large as the angular ones. This leads to extra relevant nonlinearities of the form $\delta c\partial_x\theta$, $\theta\partial_x\delta c$ in the equation for $\theta$, and $\partial_x(\delta c^2)$ and $\partial_x(\theta^2)$ in the concentration equation. These make the calculation of exact exponents in this case intractable and there is no reason, a priori, to assume that this will belong to the same universality class as the system of [9]. However, the wavevector-independent (for $\mathbf{q}\to 0$) relaxation rate of the incompressible polar model, even with concentration fluctuations, suggests that it will display long-range order in two dimensions.

## VI. ACTIVE NEMATIC MODEL WITH $\nabla\nabla : \mathbf{Q} = 0$ CONSTRAINT

In the main text and in the last section, we showed that our model in the Malthusian limit belongs to the same universality class as a a model of dry polar fluid, without concentration fluctuations, and with the constraint $\nabla\cdot\mathbf{p} = 0$. It is natural to ask whether active nematic flocks in incompressible fluids belong to the same universality class as a nematic flock with the constraint $\nabla\nabla : \mathbf{Q} = 0$. We now show that this is not the case.

The equation for the $\mathbf{Q}$ is

$$\partial_t\mathbf{Q} = (\alpha - \beta\mathbf{Q}:\mathbf{Q})\mathbf{Q} + D_Q\nabla^2\mathbf{Q} - (\nabla\nabla - \frac{1}{2}\nabla^2\mathbf{I})\Pi_Q + \boldsymbol{\sigma} \tag{41}$$

where $\boldsymbol{\sigma}$ is a traceless, symmetric non-conserving noise tensor and $\Pi_Q$ is a Lagrange multiplier that enforces the $\nabla\nabla : \mathbf{Q} = 0$ constraint. There are also nonlinearities of the form $\nabla\mathbf{Q}\nabla\mathbf{Q}$ and $\mathbf{Q}\nabla\nabla\mathbf{Q}$, but they will be irrelevant to the point we will be making.

We look at fluctuations about a phase ordered along $\hat{x}$:

$$\mathbf{Q} = \mathbf{Q}^0 + \delta\mathbf{Q} = \begin{pmatrix} Q^0_{xx} & 0 \\ 0 & -Q^0_{xx}\end{pmatrix} + \begin{pmatrix}\delta Q_{xx} & \delta Q_{xy} \\ \delta Q_{xy} & -\delta Q_{xx}\end{pmatrix}. \tag{42}$$

The constraint $\nabla\nabla : \mathbf{Q} = 0$ implies that

$$(q_x^2 - q_y^2)\delta Q_{xx} + 2q_xq_y\delta Q_{xy} = 0 \implies \delta Q_{xx} = \frac{2q_xq_y}{q_y^2 - q_x^2}\delta Q_{xy}. \tag{43}$$

The equations for linear fluctuations about this steady state are

$$\partial_t\delta Q_{xx} = -2\alpha\delta Q_{xx} + D_Q\nabla^2\delta Q_{xx} - \frac{1}{2}(\partial_x^2 - \partial_y^2)\Pi_Q + \sigma_{xx} \tag{44a}$$

$$\partial_t\delta Q_{xy} = D\nabla^2\delta Q_{xy} - \partial_x\partial_y\Pi_Q + \sigma_{xy}. \tag{44b}$$

Now we eliminate $\Pi_Q$ using the projector

$$\mathcal{P}_{ijkl} = \frac{1}{2}\left(\delta_{ik}\delta_{jl} + \delta_{il}\delta_{jk} - \delta_{ij}\delta_{ik}\delta_{jl}\right) - \frac{2q_iq_jq_kq_l}{q^4} + \frac{q_kq_l}{q^2}\delta_{ij}. \tag{45}$$

Since $Q_{xx}$ and $Q_{xy}$ are related, we need to write the equation for only one of them. We choose to write:

$$\partial_t \delta Q_{xy} = -8\alpha \frac{q_x^2 q_y^2}{q^4}\delta Q_{xy} - D_Q q^2 \delta Q_{xy} + \mathcal{P}_{xyij}\sigma_{ij}. \tag{46}$$

From this,

$$\delta Q_{xy} = \frac{\mathcal{P}_{xyij}\sigma_{ij}}{-i\omega + 2\alpha\left(\frac{2q_xq_y}{q^2}\right)^2 + D_Q q^2} \tag{47}$$

from which, we can calculate the equal time correlator,

$$\langle|\delta Q_{xy}(\mathbf{q},t)|^2\rangle = \frac{\Delta\cos^2(2\phi)}{2\alpha\sin^2(2\phi) + D_Q q^2} \tag{48}$$

where $\Delta$ is the noise strength and $\phi$ is the angle between the wavevector $\mathbf{q}$ and the ordering direction $\hat{x}$. Now using arguments similar to [9], we see that this has long-range order in two-dimensions. This also implies that the constraint $\nabla\nabla : \mathbf{Q} = 0$ leads to a system-size-independent relaxation-rate for angular fluctuations, similar to polar flocks with the constraint $\nabla \cdot \mathbf{p} = 0$. This bears no similarity to the apolar flocks in incompressible fluids on substrates whose dynamics we worked out in a separate paper [2], and which has only quasi-long-ranged order in two-dimensions and where the relaxation-rate of angular fluctuations vanish as $1/L^2$ for a system of size $L$.

## VII. DERIVATION OF TWO-DIMENSIONAL EQUATIONS FROM THREE-DIMENSIONAL CONFINED FLUID EQUATIONS

In this section we derive the effective equations for a suspension of polar swimmers in a fluid confined between two parallel plates separated by a distance $h$. We assume that the two plates impose strong-anchoring conditions on the filaments, no-slip, no-penetration boundary conditions on the velocity field and no-flux boundary condition on the concentration field. We start with the standard three-dimensional equations for the number density $\bar{c}(\mathbf{x},t)$, the polarisation vector $\bar{\mathbf{p}}(\mathbf{x},t)$ of the filaments and the velocity field $\bar{\mathbf{u}}(\mathbf{x},t) = (\bar{\mathbf{u}}_\perp, \bar{v}_z)$, as functions of three-dimensional position $\mathbf{x}$ and time $t$. We then average over the thickness of the film to get effective equations of motion valid for in-plane scales $L \gg h$ and show that to lowest order in in-plane gradients, they correspond to Eq.(1), (2) and (3) of the main text. In the first subsection we present a somewhat heuristic calculation in which we *assume* a profile of the polarisation and the velocity along the thin direction that is independent of the velocity. In the second subsection we calculate the in-plane orientational dynamics of the polarisation through a more rigorous calculation, without these assumptions, in a fixed-spin model (with a constant magnitude of the three-dimensional polarisation vector) and for small activities.

### A. General considerations and heuristic derivation

We start with the three-dimensional dynamical equations for a polar fluid. The concentration has a standard continuity equation:

$$\partial_t \bar{c} = -\bar{\nabla}\cdot\left(v_p\bar{c}\bar{\mathbf{p}} - \bar{D}_c\bar{\nabla}\bar{c}\right) \tag{49}$$

where the first term on the right in (49) describes the current generated by the active propulsion of the swimmers and the second normal diffusion.

The dynamical equation for the polar order parameter [1, 4] reads

$$\partial_t\bar{\mathbf{p}} + \bar{\mathbf{u}}\cdot\bar{\nabla}\bar{\mathbf{p}} + \bar{\lambda}_a\bar{\mathbf{p}}\cdot\bar{\nabla}\bar{\mathbf{p}} - \bar{\boldsymbol{\omega}}\times\bar{\mathbf{p}} = -\bar{\lambda}\bar{\mathbf{p}}\cdot\bar{\mathbf{U}} + \bar{\lambda}_1\bar{\nabla}^2\bar{\mathbf{u}} - \frac{\delta\bar{\mathcal{H}}}{\delta\bar{\mathbf{p}}}, \tag{50}$$

where $\bar{\mathbf{U}}$ is the symmetric parts of $\bar{\nabla}\bar{\mathbf{u}}$ and $\bar{\boldsymbol{\omega}} = (1/2)\bar{\nabla} \times \bar{\mathbf{u}}$ respectively and

$$\bar{\mathcal{H}} = \int d^3\mathbf{x} \left[ \frac{\bar{\alpha}}{2}\bar{\mathbf{p}}^2 + \frac{\bar{\beta}}{4}\bar{\mathbf{p}}^4 + \frac{\bar{K}}{2}\left(\bar{\nabla}\bar{\mathbf{p}}\right)^2 + \bar{\gamma}_p \bar{\mathbf{p}} \cdot \bar{\nabla}\bar{c} + c \ln c \right] \tag{51}$$

is a standard free energy functional governing the thermodynamics and relaxation in the absence of activity, with $\alpha$, a function of the local concentration $\bar{c}$ of active filaments, governing the onset of polar ordering, $\bar{K}$ is a rigidity which penalises local deviations away from uniform polar order, and $\bar{\gamma}_p$ couples orientation to concentration gradients. The second and third terms on the L.H.S. of (50) denote advection by the hydrodynamic velocity and active advection due to local polarization, respectively [1] i.e. passive motion with the flow and active swimming with respect to the flow. The last term on L.H.S. shows how the polarization vector will transform under a rigid rotation. The first two terms with coefficients $\bar{\lambda}$ and $\bar{\lambda}_1$ on R.H.S. are the standard terms due to flow orientation coupling encode the tendency of the polar order parameter to align with a flow gradient. Last term on the RHS of (50) encodes the physics of relaxation of the polarisation to its equilibrium value, in absence of activity.

The hydrodynamic velocity is determined by the Stokes equation $\bar{\nabla} \cdot \bar{\boldsymbol{\sigma}} = 0$ along with the incompressibility condition $\bar{\nabla} \cdot \bar{\mathbf{u}} = 0$. The total stress $\bar{\boldsymbol{\sigma}} = \bar{\boldsymbol{\sigma}}^p + \bar{\boldsymbol{\sigma}}^a$ consists of a passive part

$$\bar{\boldsymbol{\sigma}}^p = 2\bar{\eta}\bar{\mathbf{U}} - \bar{\Pi}\mathbf{I} - 2\bar{\lambda}\left[\bar{\mathbf{p}}\frac{\delta\bar{\mathcal{H}}}{\delta\bar{\mathbf{p}}}\right]^{ST} + \bar{\lambda}_1\left[\bar{\nabla}\frac{\delta\bar{\mathcal{H}}}{\delta\bar{\mathbf{p}}}\right]^{ST} + 2\left[\bar{\mathbf{p}}\frac{\delta\bar{\mathcal{H}}}{\delta\bar{\mathbf{p}}}\right]^{A} - \bar{\nabla}\bar{\mathbf{p}} \cdot \frac{\partial\bar{\mathrm{h}}}{\partial(\bar{\nabla}\bar{\mathbf{p}})}, \tag{52}$$

where the last term is the Ericksen stress [11] with $\bar{\mathrm{h}}$ being the free energy density, i.e., the integrand in (51), and the reappearance in (52) of $\lambda$, $\lambda_1$ from (50) is a consequence of the (Onsager) antisymmetry of reversible kinetic coefficients. The active stress

$$\bar{\boldsymbol{\sigma}}^a = \bar{\zeta}[\bar{\mathbf{p}}\bar{\mathbf{p}}]^{ST} + \bar{\zeta}_p[\bar{\nabla}\bar{\mathbf{p}}]^{ST} \tag{53}$$

is governed by parameters $\zeta$ and, crucially, $\zeta_p$. Clearly $\zeta$ and $\zeta_p$ carry very different information. The sign of $\zeta$ determines the contractile or extensile character of the active stresses, while $\zeta_p$ [5] characterises the fore-aft symmetry of the flow around, and hence the motility of, an elementary active object, i.e., the degree to which it is a mover, not merely a shaker [7] characterising the leading contributions with apolar and polar character respectively.

Equations (49), (50), (52), and (53) constitute a complete description of an active polar system. This is our starting point for the construction of the effective two dimensional description. We supplement these equations with appropriate boundary conditions and integrate over the thickness to find an effective set of two-dimensional equations. Assuming for simplicity a Poiseuille profile for the velocity field, with a given mid-plane horizontal velocity $\bar{\mathbf{u}}_0$ and no slip on the bounding surfaces at $z = 0$ and $z = h$ we get an in-plane velocity

$$\bar{\mathbf{u}}_\perp(z) = \frac{4}{h^2}\bar{\mathbf{u}}_0(zh - z^2). \tag{54}$$

Thus, the $z$-averaged viscous force density is $(8\bar{\eta}/h^2)\bar{\mathbf{u}}_0$ and the $z$-averaged velocity is $\mathbf{u} = (2/3)\bar{\mathbf{u}}_0$, and

$$\frac{1}{h}\int_0^h \bar{\eta}\bar{\nabla}^2\bar{\mathbf{u}}_\perp dz = -\Gamma\mathbf{u} + O(\epsilon^2), \tag{55}$$

where

$$\Gamma = 12\bar{\eta}/h^2. \tag{56}$$

Though we have assumed a Poiseuille profile for the flow, only the numerical coefficient in the definition of $\Gamma$ can change if other kinds of flows (for instance, plug flow) are considered. The three-dimensional incompressibility constraint also translates to $\nabla \cdot \mathbf{u}$, where $\nabla$ is the two-dimensional gradient operator. For the polarisation field, let us consider walls favouring normal alignment of the polar filaments. The antagonistic boundary conditions $\bar{\mathbf{p}}|_{z=0} = \hat{z}$ and $\bar{\mathbf{p}}|_{z=h} = -\hat{z}$, shown in Fig. 1, are then natural and force the bulk polarisation $\bar{\mathbf{p}}$ to have a non-trivial $z$-dependence. Deep in the ordered phase, where $|\bar{\mathbf{p}}|$ is constrained to be a constant, this implies that $\bar{\mathbf{p}}_\perp$ will also have a $z$-dependence. In this case, the lowest order polar active term present in the velocity equation, $\int_0^h dz\partial_z^2\bar{\mathbf{p}}_\perp$, will have a $z$-averaged value proportional to $\mathbf{p}$ – the $z$-averaged value of $\bar{\mathbf{p}}_\perp$, with a coefficient $\upsilon$. We show this explicitly, for a specific case in the next subsection. However, this is easy to see intuitively by analogy to the arguments presented for $\bar{\mathbf{u}}$ (or by assuming a parabolic profile for $\bar{\mathbf{p}}_\perp$). Note that though we have used a specific boundary condition to illustrate how $\bar{\mathbf{p}}_\perp$ can have a non-trivial $z$-dependence, this will be the case for most boundary conditions.

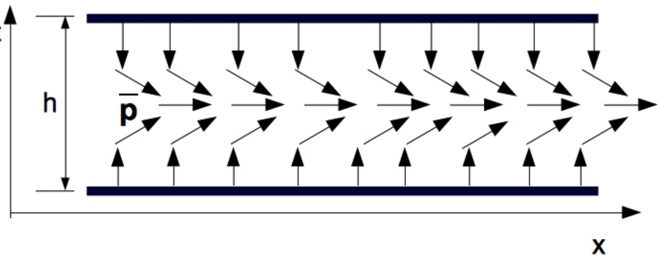


FIG. 1: Polarisation profile in a channel with boundary condition $\bar{\mathbf{p}}_{\bar{z}=0} = \hat{z}$ and $\bar{\mathbf{p}}_{\bar{z}=h} = -\hat{z}$
.

Turning to the polarisation equation we see that it contains a term proportional to $\bar{\nabla}^2\bar{\mathbf{u}}$. In a $z$-averaged description, this results in a term proportional to $\mathbf{u}$ in the polarisation equation by precisely the same argument that was used to justify the presence of the friction coefficient in the velocity equation. In particular, if the velocity has a parabolic profile, $\Lambda = 3\bar{\lambda}_1/4h^2$. We note that this contribution is purely passive: in any system without Galilean invariance, the polarisation can orient along the local velocity and not only along the local velocity gradient [8]. However, even for systems without Galilean invariance, forces must be derived from a free-energy if the system is in equilibrium. Thus, a force proportional to the local polarisation is not possible in an ordered passive system. The final equations obtained from the averaging procedure is

$$\partial_t \mathbf{p} + \mathbf{u}\cdot\nabla\mathbf{p} + \lambda_a \mathbf{p}\cdot\nabla\mathbf{p} - \boldsymbol{\omega}\times\mathbf{p} = \Lambda\mathbf{v} - \lambda\mathbf{p}\cdot\mathsf{U} - \lambda_1\nabla^2\mathbf{v} - \frac{\delta\mathcal{H}}{\delta\mathbf{p}}, \tag{57a}$$

$$\Gamma\mathbf{u} = \upsilon\mathbf{p} - \nabla\Pi + \zeta_p\nabla^2\mathbf{p} + \zeta\cdot\nabla(\mathbf{pp}) - \Lambda\frac{\delta\mathcal{H}}{\delta\mathbf{p}}, \tag{57b}$$

$$\partial_t c = -\nabla\cdot(\upsilon_p c\mathbf{p} - D_c\nabla c). \tag{57c}$$

These equations are the generalised versions (includes higher order terms) of (1), (2) and (3) of the main text.

### B. Rigorous derivation

In this section we will present a detailed derivation of the effective two-dimensional equation for a hard-spin ($|\bar{\mathbf{p}}|$ constant) polar active fluid model. In contrast to the last section, where we argued for the form of the two-dimensional equations by assuming a parabolic profile for the polarisation and the velocity for simplicity, here we will make no such assumption. We will obtain the effective dynamical equation for the fluctuation of the in-plane, thickness-averaged polarisation field, which reassuringly, will turn out to have the same form as the one obtained in the last section. We will first calculate the steady-state of the polarisation and the velocity field when the velocity field has no-slip boundary condition on both surfaces and the polarisation at the boundaries is $\bar{\mathbf{p}}|_{z=0} = \hat{z}$ and $\bar{\mathbf{p}}|_{z=h} = -\hat{z}$. Since the magnitude of the polarisation vector is fixed, $\bar{\mathbf{p}} = (\sin\Theta\cos\Psi, \sin\Theta\sin\Psi, \cos\Theta)$, where $\Theta$ is the polar angle and the $\Psi$ is the azimuthal angle. We look for a steady state with $\Psi = 0$. By scaling in-plane lengths by $L$ and $z$ by $h$, we see that $\bar{\nabla}_\perp$ is $\epsilon$ times smaller than $\partial_z$, where $\epsilon = h/L$. To find the steady-state, we will expand the dynamical equations to the lowest order in $\epsilon$. With these considerations, the Stokes equation turns into

$$-\frac{d^2\bar{u}_x}{dz^2} = \bar{f}_x(z), \tag{58}$$

where

$$\bar{f}_x(z) = \frac{\bar{\zeta}}{\bar{\eta}}\cos 2\Theta\frac{d\Theta}{dz} + \frac{\bar{\zeta}_p}{\bar{\eta}}\cos\Theta\frac{d^2\Theta}{dz^2} - \frac{\bar{\zeta}_p}{\bar{\eta}}\sin\Theta\left(\frac{d\Theta}{dz}\right)^2. \tag{59}$$

along with the boundary condition $\bar{u}_x = 0$ at $z = 0$ and $z = h$ and

The $\Theta$ equation in the steady-state is

$$-\bar{\Gamma}_p\bar{K}\frac{d^2\Theta}{dz^2} = \frac{1-\bar{\lambda}}{2}\cos^2\Theta\frac{d\bar{u}_x}{dz} + \bar{\lambda}_1\cos\Theta\frac{d^2\bar{u}_x}{dz^2} \tag{60}$$

The coupled equation above is difficult to solve in general. However, the equations become tractable if we assume that the activity is small: $\bar{\zeta} \to 0$ and $\bar{\zeta}_p \to 0$. In this case, we can solve the equations perturbatively in activity parameters, with the boundary condition $\Theta = \pi/2$ at $z = h$ and $\Theta = -\pi/2$ at $z = 0$. At zeroth order in the activity parameters, the solution is trivial $\Theta^0 = z\pi/h - \pi/2$. Replacing these in the equations for the angle and velocity fields, we find the equation for the angle field correct to the first order in activity and consider planar perturbation about this steady state. The linearised perturbation equation for $\Psi$ is

$$\sin^2\Theta[\partial_t\Psi + \bar{u}_x^0\partial_x\Psi] = \frac{1-\bar{\lambda}}{2}\sin 2\Theta\left[\Psi\frac{d\bar{u}_x^0}{dz} + \partial_z\bar{u}_y)\right] + \frac{\sin^2}{2}\Theta\left[(1-\bar{\lambda})\partial_x\bar{u}_y - (\bar{\lambda}+1)\partial_y\bar{u}_x\right] + \bar{\lambda}_1\Psi\sin\Theta\frac{d^2\bar{u}_x^0}{dz^2} + \bar{\lambda}_1\sin\Theta\bar{\nabla}^2\bar{u}_y + \bar{K}\bar{\Gamma}\left[\sin^2\Theta\bar{\nabla}^2\Psi + 2\sin 2\Theta(\partial_z\Psi)\frac{d\Theta}{dz}\right] \quad (61)$$

with the boundary conditions $\Psi = 0$ at $z = h$ and $z = 0$ and where $u_x^0$ is the $z$ dependent steady velocity along $x$. We now use an ansatz

$$\Psi = \theta(x,y,t) + \epsilon^2\nu(x,y,z,t) \quad (62)$$

where $\theta$ is the $z$ averaged $\Psi$ field. The in-plane Fourier-transformed velocity perturbation equations are

$$-\epsilon^2q^2\bar{\mathbf{u}}_q(z) + \partial_z^2\bar{\mathbf{v}}_q(z) = -\epsilon\frac{1}{\bar{\eta}}(\bar{\mathbf{I}} - \hat{\mathbf{q}}\hat{\mathbf{q}})\cdot\bar{\mathbf{f}}_q(z), \quad (63)$$

where $\bar{\mathbf{f}}_q(z) = \int d^2\mathbf{r}e^{i\mathbf{q}\cdot\mathbf{r}}\bar{\mathbf{f}}(\mathbf{r},z)$ where, to lowest order in activity, and using (62)

$$\bar{f}_x(\mathbf{r},z) = \bar{\zeta}\left[\epsilon\sin^2\Theta\partial_y\theta\right] \quad (64)$$

$$\bar{f}_y(\mathbf{r},z) = \bar{\zeta}\left[\cos 2\Theta\frac{d\Theta}{dz}\theta + \epsilon\sin^2\Theta\partial_x\theta\right] + \bar{\zeta}_p\left[\theta\cos\Theta\epsilon^{-1}\frac{d^2\Theta}{dz^2} - \sin\Theta\epsilon^{-1}\left(\frac{d\Theta}{dz}\right)^2\theta + \sin\Theta\epsilon\bar{\nabla}_\perp^2\theta\right] \quad (65)$$

We solve for the velocity using the Green's function

$$G_q(z,z') = \frac{1}{q_e\,\sinh(q_eh)}\sinh(q_ez)\sinh[q_e(z'-h)] \qquad z < z'$$
$$G_q(z,z') = \frac{1}{q_e\,\sinh(q_eh)}\sinh(q_ez')\sinh[q_e(z-h)] \qquad z > z', \quad (66)$$

where $q_e = q/\epsilon$, and $z$-average (61) to obtain an effective equation for $\theta$. The detailed form of the coefficients are complicated and not very illuminating, but the equation has the form

$$\partial_t\theta + iq_xu_x^0\theta = s_1\frac{-q_y^2}{q^2}\theta + \left[\frac{1-\bar{\lambda}}{2}iq_xu_y - \frac{1+\bar{\lambda}}{i}q_yu_x\right] - \bar{\lambda}_1q^2u_y - \bar{\Gamma}_p\bar{K}q^2\theta, \quad (67)$$

The value of $s_1$ can be expressed in terms of the previous coefficients. Though its explicit form is not very illuminating [10], it should be noted that it is $\mathcal{O}(q^0)$. Defining $\phi$ as the angle between the wavevector and $x$, we see that the zeroth order to wavevector,

$$\partial_t\theta \sim -(\sin^2\phi)\theta \quad (68)$$

as claimed in the main text. We highlight the crucial role of incompressibility in producing this zeroth order damping. If the fluid is made compressible, where $\bar{\nabla}^2\bar{\mathbf{u}} = -\bar{\mathbf{f}}$, the $z$ dependent part of $f_y$ is $\theta$ times the $z$ dependent part of $f_x$. Using this in (61) we see that all the terms that depend on $z$ derivatives cancel and the (61) transforms to

$$\sin^2\Theta[\partial_t\Psi + iq_xu_x^0\Psi] = \sin^2\Theta\left[\frac{1-\bar{\lambda}}{2}iq_xu_y - \frac{1+\bar{\lambda}}{i}q_yu_x\right] - \sin\Theta\bar{\lambda}_1q^2u_y - \bar{\Gamma}_p\bar{K}\sin^2\Theta q^2\Psi \quad (69)$$

This equation upon $z$ averaging does not produce a zeroth-order in wavevectors damping of $\theta$ due to the short-ranged nature of the hydrodynamic interactions in a compressible fluid. This completes our demonstration that the transverse fluctuations of an incompressible polar fluid confined between two plates is damped at zeroth-order in wavevectors, for arbitrarily small activity, as we argued for in the main text.

## VIII. INCOMPRESSIBLE-COMPRESSIBLE CROSSOVER

In this section we will present the detailed calculation that demonstrates our conclusions regarding superstability and non-giant fluctuations are also applicable up to very large length scales in weakly compressible systems such as fluid-less collections of motile particles or active polar rods in a dense bead medium. As discussed in the main text, for this we introduce the additional dynamics of the overall density field $\rho$, $\partial_t \rho = -\nabla \cdot (\rho \mathbf{u})$, which in a perfectly incompressible system would lead to the constraint $\nabla \cdot \mathbf{u} = 0$. The pressure in the force balance equation is now determined by an equation of state $\Pi = \delta\rho/(\chi\rho_0)$ where $\delta\rho$ is the deviation from the mean density $\rho_0$. The equation for the polarisation field remains unmodified due to the explicit inclusion of $\rho$. In this section we will ignore the usual concentration field $c$ associated with the concentration of active particles in a two-fluid model that we considered in the main text for the sake of clarity. We have checked this does not affect the crossover to the incompressible limit that we wish to highlight. Furthermore, if we consider a Malthusian flock, $c$ is not a hydrodynamic variable and if the compressible system that we wish to describe has only one component, such as a Toner-Tu flock, there is no $c$. Eliminating the velocity field in the overdamped limit in terms of the polarisation and $\rho$ fluctuations and integrating out the fluctuations of the polarisation magnitude, we obtain the coupled linearised dynamics of $\rho$ and $\theta$:

$$\partial_t \rho = -iv_\rho q_x \rho - \frac{1}{\chi\rho_0\Gamma} q^2 \rho - i\frac{w}{\Lambda} p_0 q_y \theta + \xi_c \tag{70}$$

$$\partial_t \theta = -iv_1 q_x \theta - K_p(\phi) q^2 \theta - i\frac{\Lambda}{\chi\rho_0\Gamma p_0} q_y \rho + \xi \tag{71}$$

where $v_1$ is the speed at which the polarisation fluctuations are advected and $\xi_c$ and $\xi$ are conserving and nonconserving Gaussian white noises respectively:

$$\langle \xi(\mathbf{r}, t)\xi(\mathbf{r}', t')\rangle = 2B\delta(\mathbf{r} - \mathbf{r}')\delta(t - t'). \tag{72}$$

$$\langle \xi_c(\mathbf{r}, t)\xi_c(\mathbf{r}', t')\rangle = -2B_c\nabla^2\delta(\mathbf{r} - \mathbf{r}')\delta(t - t'). \tag{73}$$

Equations (70) and (71) together lead to the standard Toner-Tu waves. To examine the $\chi \to 0$ limit, we now calculate the two-point correlator of the angle fluctuations:

$$\langle \theta(q, \omega)\theta(-q, -\omega)\rangle = \frac{2B}{|K_p q^2 + i\omega - iv_1 q\cos\phi + \{q^2 w \sin^2\phi/(q^2 + i\chi\rho_0\Gamma\omega - iqv_\rho\chi\rho_0\Gamma\cos\phi)\}|^2} \tag{74}$$

In the incompressible limit i.e., when $\chi \to 0$, this reduces to

$$\langle \theta(q, \omega)\theta(-q, -\omega)\rangle = \frac{2B}{|K_p q^2 + i\omega - iv_1 q\cos\phi + w\sin^2\phi|^2} \tag{75}$$

From this, we find the equal time correlator of the angular fluctuations:

$$\langle \theta_q(t)\theta_{-q}(t)\rangle = \frac{B}{K_p(\phi)q^2 + w\sin^2\phi} \tag{76}$$

Thus, we have shown the emergence of the wavevector-independent relaxation rate and the consequent super-stability by starting with a compressible model and taking the limit of vanishing compressibility.

We now calculate the angular static structure factor for arbitrary $\chi$ in the frame moving at a speed $v_1\hat{x}$ simplifying limit $v_1 = v_\rho$ (this considerably simplifies the algebra and the notation, but does not change any scaling or result). Defining $D_\rho = 1/\chi\rho_0\Gamma$, the angular static structure factor is

$$C_{\theta\theta} = B\frac{q^2(D_\rho + K_p) + w\sin^2\phi}{q^2(D_\rho + K_p)(K_p q^2 + w\sin^2\phi)}. \tag{77}$$

We now define the length scale $\ell^{*2} = K_p/w$, the dimensionless ratio of orientational and mass diffusivities $\tilde{\chi} = K_p/D_\rho$, the timescale $\tau^* = 1/w = \ell^{*2}/K_p$, and the non-dimensionalised wavevector $\tilde{q} = q\ell^*$ (these definitions are mildly direction-dependent since $K_p$ is a function of $\phi$ which is positive for all $\phi$). In terms of these variables, the full static structure factor is

$$C_{\theta\theta} = \frac{B\tau^*}{\tilde{q}^2 + \sin^2\phi}\left[1 + \frac{\tilde{\chi}}{\tilde{\chi} + 1}\frac{\sin^2\phi}{\tilde{q}^2}\right] \tag{78}$$

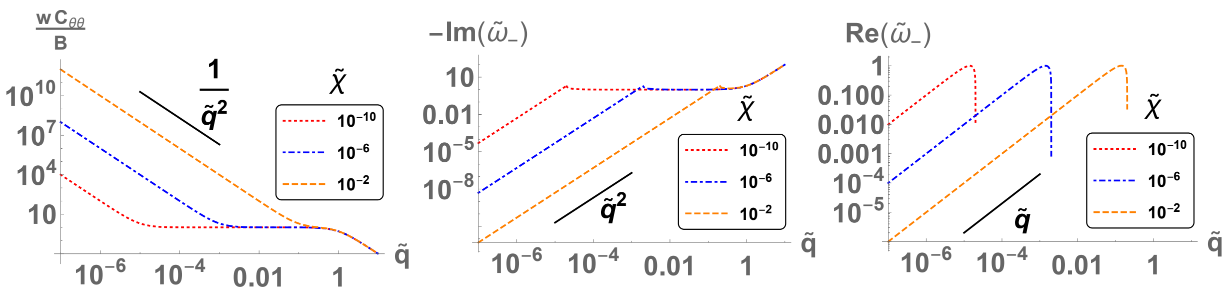


(a) (b) (c)

FIG. 2: The nondimensionalised angular static structure factor (a), $\mathrm{Im}(\tilde{\omega}_-)$ (b) and $\mathrm{Re}(\tilde{\omega}_-)$ (c) for $\phi = \pi/2$ for various values of $\tilde{\chi}$ plotted as function of $\tilde{q}$. The $q$-independent plateau is seen in (a) and (b) while (c) demonstrates that, as expected, the Toner-Tu waves are observed only for $\tilde{q} < \sqrt{\tilde{\chi}}$.

For small $\tilde{\chi}$, this yields the crossover scale $L^* = \ell^*/\sqrt{\tilde{\chi}} = \sqrt{D_\rho/w} = 1/\sqrt{\chi\rho_0 w\Gamma}$, at which the usual $1/q^2$ scaling of the angular static structure factor is obtained. For $\phi \approx \pi/2$, there is a $q$-independent plateau for wavevectors $1/L^* < q < 1/\ell^*$. This plateau shrinks to 0 as $\phi \to 0$.

We now calculate the eigenfrequencies implied by (70) and (71), non-dimensionalising them as $\tilde{\omega} = \omega\tau^*$. The eigenfrequencies in these units are

$$\tilde{\omega}_\pm = -i\frac{\tilde{q}^2}{2}\left[\frac{\tilde{\chi}+1}{\tilde{\chi}} \pm \frac{|1-\tilde{\chi}|}{\tilde{\chi}}\sqrt{1 - \frac{4\tilde{\chi}}{(1-\tilde{\chi})^2}\frac{\sin^2\phi}{\tilde{q}^2}}\right] \tag{79}$$

We see that when $q \gg 1/L^*$, both eigenfrequencies are purely imaginary for $\phi \approx \pi/2$ while for $q < 1/L^*$, they acquire a propagating (real) part. One of the two eigenfrequencies, diverges in the $\tilde{\chi} \to 0$ limit. The eigenvector associated with this eigenvalue is purely along $\rho$ in this limit implying that this describes the fast relaxation of density to its steady-state value in the incompressible limit. The other eigenvalue becomes

$$\tilde{\omega}_- = -i(\tilde{q}^2 + \sin^2\phi). \tag{80}$$

Note that both the relaxation rates, that is $\mathrm{Im}[\tilde{\omega}_\pm]$ turn purely diffusive as soon as the discriminant in (79) turns negative, i.e., for $\tilde{q} < 2\sqrt{\tilde{\chi}}/|1-\tilde{\chi}| \approx 2\sqrt{\tilde{\chi}}$ for small $\tilde{\chi}$ along $\phi = \pi/2$. This implies that $\mathrm{Im}[\tilde{\omega}_-]$ which governs the angular relaxation has a $\tilde{q}$-independent plateau for wavevectors $1 > \tilde{q} > 2\sqrt{\tilde{\chi}}$ (Note that the $q^0$ plateau in the static structure factor persists for a slightly larger range of wavevectors, $\sqrt{\tilde{\chi}} < \tilde{q} < 1$).

We now check how the real parts of the eigenfrequencies (describing wave-like excitations) vanish $q^2 \approx \tilde{q}_0^2 = 4\tilde{\chi}/(1-\tilde{\chi})^2$. Defining $\delta q = \tilde{q} - \tilde{q}_0$, we find that (79) implies an eigenfrequency

$$\tilde{\omega}_\pm = -i\frac{\tilde{q}^2}{2}\left[\frac{\tilde{\chi}+1}{\tilde{\chi}} \pm \frac{|1-\tilde{\chi}|}{\tilde{\chi}}\sqrt{\frac{2\delta q}{\tilde{q}_0}}\right]. \tag{81}$$

Therefore, for $\delta q < 0$, the real part of the eigenfrequencies are

$$\mathrm{Re}[\tilde{\omega}_\pm] = \pm\frac{1}{\sqrt{2}}\frac{|1-\tilde{\chi}|}{\tilde{\chi}}(\tilde{q}_0^{3/2} - 2\delta q\sqrt{\tilde{q}_0})\sqrt{\delta q} \tag{82}$$

This implies that the sound modes vanish as $\sqrt{\tilde{q}-\tilde{q}_0}$ exactly at the start of the plateau in the eigenfrequency spectrum at $\tilde{q}_0$.

We plot the angular static structure factor (78), $\mathrm{Im}(\tilde{\omega}_-)$ and $\mathrm{Re}(\tilde{\omega}_-)$ as functions of $\tilde{q}$ for various values of $\tilde{\chi}$ in Fig. 2. This completes the detailed calculation of the results regarding the range of system sizes for the observation of effectively incompressible behaviour in a compressible system. In particular, we have presented the detailed calculation leading up to Eq (9) and (10) of the main text that describes the plateaus in the static structure factor and the imaginary part of the eigenfrequency whose extent increases as $\tilde{\chi}^{-1/2}$.

---

* ananyo.maitra@u-psud.fr

† martin.lenz@u-psud.fr

[1] M. C. Marchetti et al., Rev. Mod. Phys **85**, 1143 (2013)
[2] A. Maitra et al. Proc. Natl. Acad. Sci. USA **115**, 6934 (2018)
[3] S. Ramaswamy, Statphys, Lyon
[4] W. Kung, M. C. Marchetti and K. Saunders, Phys. Rev. E **73**, 031708 (2006)
[5] L. Giomi, T. B. Liverpool, M. C. Marchetti Phys. Rev. E **81**, 051908 (2010)
[6] H.A. Stone, in Nonlinear PDEs in Condensed Matter and Reactive Flows, NATO Science Series C: Mathematical and Physical Sciences, **569**, H. Berestycki and Y. Pomeau eds., Kluwer Academic, Dordrecht, The Netherlands (2002); A. Oron, S.H. Davis, S.G. Banko , Rev. Mod. Phys. **69**, 931 (1997)
[7] Y. Hatwalne et al. Phys. Rev. Lett **92**, 118101 (2004)
[8] N. Kumar et al., Nat. Comm. **5**, 4688 (2014)
[9] L. Chen, C-F. Lee, J. Toner, Nat. Comm **7**, 12215 (2016)
[10] See A Maitra, PhD thesis, Indian Institute of Science (2014) for the algebraic details.
[11] P. G. de Gennes, J. Prost, The Physics Of Liquid Crystals, Clarendon Press (1995)
[12] J. Toner, Phys. Rev. Lett. **108**, 088102 (2012)
[13] S. Ramaswamy, G. F. Mazenko, Phys Rev A **26**, 1735 (1982)
